# Supplementary material for: Transformation of spin current by antiferromagnetic insulators
Source: arXiv:1511.05785 source file (2016-03-16)
Supplement: Supplementary file 1 [file ArxivAFMSupplResubmFin.pdf]

# Transformation of spin current by antiferromagnetic insulators. Supplementary materials

Roman Khymyn,[1,*] Ivan Lisenkov,[1,2] Vasil S. Tiberkevich,[1] Andrei N. Slavin,[1] and Boris A. Ivanov[3]

[1]*Department of Physics, Oakland University, Rochester, Michigan 48309, USA*
[2]*Institute of Radio-engineering and Electronics of RAS, Moscow 125009, Russia*
[3]*Institute of Magnetism, NASU and MESYSU, Kiev 03142, Ukraine*

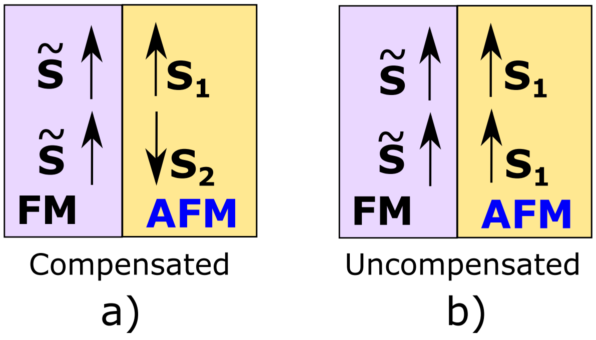


FIG. S.1. Two types of FM/AFM interface: a) totally compensated AFM boundary with zero magnetization, b) totally uncompansated AFM boundary.

## ENERGY FLUX

In the FM/AFM/Pt layered structure the magnetization precession in the ferromagnetic (FM) layer excites spin dynamics in the antiferromagnetic (AFM) layer.

It is obvious, that, besides the transfer of spin current from the FM to AFM layer, there is also a *flux of energy* from the FM to the AFM layer. This flux of energy $\Pi$ can be found from the Lagrangian Eq. (2) by applying the Noether theorem, and has the following form:

$$\Pi = 8\frac{\mu c^3\omega^2}{\beta}\sum_{i=1,2}\frac{a_i^2}{(c^2/\beta^2-\omega^2\lambda_i^2)\,(1+\cosh 2d/\lambda_i)} \tag{S.1}$$

Here and below all the notation is the same as in the main text of the paper.

As one can see from Eq. (S.1), the flux of energy does not depend on both the spatial coordinate $y$ inside the AFM and the phase shift $\phi$ between the excited evanescent AFM modes. Therefore, the FM layer is a source and Pt layer is a receiver of the energy coming from the FM layer, and this flux of energy is not transformed inside the AFM layer (besides negligible Gilbert damping, see Fig. 4.).

At the same time,the situation with the spin current is quite different. Due to the anisotropy of the AFM layer the angular momentum is not conserved inside the magnetic subsystem of the AFM layer, and, therefore, there appears a flux of angular momentum between the spin subsystem and the lattice of the AFM.

Thus, at certain parameters of the spin dynamics in the AFM it is possible to create a flux of angular momentum from the lattice into the spin subsystem. In this case it is possible to get the output spin current that is larger than the input one, but, obviously, the flux of energy at the output will never be larger than at the input.

The efficiency of the spin transfer through the AFM layer can be characterized by the ratio of the spin current at the output of the AFM layer to the energy losses of the FM layer. Thus, we can introduce the value $S_{\text{eff}} = \omega P|_{y=d}/\Pi$, which is defined as the ratio of the transferred angular momentum to the energy flux, and, therefore, can be interpreted as "effective spin" of the spin transfer.

As one can see, the energy flux is the sum of the energies of both evanescent AFM modes, and has the form $\Pi = A_1a_1^2 + A_2a_2^2$, while the spin current depends on the product of the modes' amplitudes $P = C|a_1a_2|$. Thus, the effective spin has the maximum value $S_{\text{eff}} = C/2\sqrt{A_1A_2}$. Maximizing this value with respect to the phase shift $\phi$ between the excited evanescent AFM modes one can obtain the maximum efficiency of the spin transfer $S_{\text{eff}}^{\max} = 1$.

Physically the difference in the behavior of the energy and the spin flux originates from the symmetries of the Lagrangian (2). The flux of energy is defined by the infinitesimal shifts of the Lagrangian in *time*, which are uniform in an absence of damping, resulting in an energy conservation. In contrast, the flux of the angular momentum is defined by the infinitesimal *rotations* of the Lagrangian (2). Obviously, the rotation operation does not transfer the system to itself in case of a bi-axial anisotropy, and the angular momentum in the spin system of the anisotropic AFM is not conserved.

## AFM DYNAMICS DRIVEN BY THE MAGNETIZATION PRECESSION IN THE FM LAYER

Let us consider the excitation of dynamics in the AFM by the processes happening at AFM/FM interface. We assume, that the magnetic coupling between the FM and AFM is of the exchange origin and, therefore, is strongly localized at the AFM/FM interface. The spins existing at the AFM boundary can belong either to the different sublattices of the AFM, as shown in Fig. S.1 a), or to the same one (see Fig. S.1 b). In the first case the AFM

has no static magnetization at the interface and will be called below a *compensated* AFM, while in the second case, the boundary of the AFM is magnetized, and such AFM will be called *uncompensated*.

The exchange coupling between the AFM and FM creates an additional term in the energy of the AFM. In the case of a *compensated* AFM the additional energy is expressed as $\Delta E = \sum J_s\left(\tilde{\mathbf{S}}\cdot\mathbf{S_1} - \tilde{\mathbf{S}}\cdot\mathbf{S_2}\right)$, where $J_s$ is the interface exchange integral, $\tilde{\mathbf{S}}$ is the FM spin at the interface, and the summation is taken over the whole FM/AFM interface.

After the transition to a continuum limit and taking into account the relation Eq. (1) in the main text of the paper, one can write an additional term in the Lagrangian Eq. (2) as $E_s(\mathbf{m}_{\rm FM}\cdot\mathbf{m})\delta(y)$, where $\mathbf{m}_{\rm FM}$ is the unit vector defining the magnetization direction in the FM layer, $E_s$ is the density of the surface exchange energy describing FM/AFM coupling, and $E_s$ is proportional to the exchange integral $J_s$: $E_s \propto J_s$ .

Considering the case of an *uncompensated* boundary of the AFM one can find the additional coupling energy as $\Delta E = \sum 2J_s\tilde{\mathbf{S}}\cdot\mathbf{S_1}$, which lead to the term $E_s[\mathbf{m}_{\rm FM}\cdot(\mathbf{m}+\mathbf{l})]\delta(y)$. Usually, the AFM boundary is *partially uncompensated*, and we introduce the phenomenological parameter $\alpha\in[0..1]$, which describes the *degree of the AFM non-compensation* at the FM/AFM interface.

Using the well-known expression for the AFM magnetization [16,18,19]:

$$\mathbf{m} = \frac{1}{\gamma H_{ex}}[\mathbf{l}\times\frac{\partial\mathbf{l}}{\partial t}] \tag{S.2}$$

it is easy to obtain the Lagrange equations describing the spin dynamics inside the AFM:

$$2\mu\left\{[\mathbf{l}\times\frac{\partial^2\mathbf{l}}{\partial t^2}] - c^2[\mathbf{l}\times\frac{\partial^2\mathbf{l}}{\partial x^2}]\right\} - [\mathbf{l}\times\frac{\partial W_a}{\partial\mathbf{l}}] =$$
$$= E_s\delta(y)\left\{\alpha[\mathbf{l}\times\mathbf{m}_{\rm FM}] + \left[\mathbf{l}\times\frac{1}{\gamma H_{ex}}\left(2\left[\frac{\partial\mathbf{l}}{\partial t}\times\mathbf{m}_{\rm FM}\right] + \left[\mathbf{l}\times\frac{\partial\mathbf{m}_{\rm FM}}{\partial t}\right]\right)\right]\right\} \tag{S.3}$$

Since vector $\mathbf{l}$ in the ground state is directed along the vector $\mathbf{e}_3$, we can in the case of a negligibly small dissipation write the dynamic equations for only two components $l_1$ and $l_2$ of the vector $\mathbf{l}$. These equations have the form analogous to the form of the dynamic equation (3) in the main text of the paper:

$$\frac{\partial^2 l_1}{\partial t^2} - c^2\frac{\partial^2 l_1}{\partial y^2} + \omega_1^2 l_1 = \frac{E_s\delta(y)}{2\mu}\left[\alpha(\mathbf{m}_{\rm FM}\cdot\mathbf{e}_1) + \frac{1}{\gamma H_{ex}}\left[2\frac{\partial l_2}{\partial t}(\mathbf{m}_{\rm FM}\cdot\mathbf{l}) + l_2\left(\frac{\partial\mathbf{m}_{\rm FM}}{\partial t}\cdot\mathbf{l}\right)\right] - \left(\frac{\partial\mathbf{m}_{\rm FM}}{\partial t}\cdot\mathbf{e}_2\right)\right] \tag{S.4}$$
$$\frac{\partial^2 l_2}{\partial t^2} - c^2\frac{\partial^2 l_2}{\partial y^2} + \omega_2^2 l_2 = \frac{E_s\delta(y)}{2\mu}\left[\alpha(\mathbf{m}_{\rm FM}\cdot\mathbf{e}_2) - \frac{1}{\gamma H_{ex}}\left[2\frac{\partial l_1}{\partial t}(\mathbf{m}_{\rm FM}\cdot\mathbf{l}) + l_1\left(\frac{\partial\mathbf{m}_{\rm FM}}{\partial t}\cdot\mathbf{l}\right)\right] - \left(\frac{\partial\mathbf{m}_{\rm FM}}{\partial t}\cdot\mathbf{e}_1\right)\right] \tag{S.5}$$

The above equations are the equations describing dynamics of an oscillatory system driven by an external force $\mathbf{f}(t)\delta(y)$, where $\mathbf{f}(t)$ are the right-hand-side parts of the above equations.

We consider the harmonic driving force and, therefore, $\mathbf{m}_{\rm FM}\propto e^{-i\omega t}$. In this case, when $\omega<\omega_1,\omega_2$ the solutions of these equations are the evanescent modes that exponentially decay with the increase of the coordinate $y$ inside the AFM. These solutions are given explicitly by Eq. (4) in the main paper.

To obtain the values of the amplitudes $a_1$ and $a_2$ in the Eq. (6) we consider a generic case, when the magnetization in the FM layer is parallel to the AFM vector $\mathbf{m}_{\rm FM}=\mathbf{e_3}$. Then, the precessional motion of the magnetization in the FM layer can be expressed as:

$$\begin{aligned}\mathbf{m}_{\rm FM}\cdot\mathbf{e}_1 &= \sin\theta\sin\omega t\\ \mathbf{m}_{\rm FM}\cdot\mathbf{e}_2 &= \sin\theta\cos\omega t,\end{aligned} \tag{S.6}$$

where $\theta$ is the magnetization precession angle in the FM. In this case, the amplitudes $a_1$ and $a_2$ of the two evanescent modes $l_1$, $l_2$ have the form:

$$|a_1| = \gamma\frac{E_s}{2M_s}\frac{|\omega+\alpha\gamma H_{ex}|}{c\sqrt{\omega_1^2-\omega^2}}\sin\theta, \tag{S.7}$$

$$|a_2| = \gamma\frac{E_s}{2M_s}\frac{|-\omega+\alpha\gamma H_{ex}|}{c\sqrt{\omega_2^2-\omega^2}}\sin\theta, \tag{S.8}$$

and the phase shift is $\phi=\pi/2$.

## ISHE VOLTAGE IN THE PT LAYER

Now, it is easy to find the spin current at the AFM/Pt interface for the different thicknesses of the AFM layer, using Eq. (10) in the main text, and to calculate the voltage of produced in the Pt layer by ISHE. The ISHE voltage can be written as [23]:

$$V_{\text{ISHE}} = \rho \Theta_{SH} w \left(\frac{2e}{\hbar}\right) \frac{\lambda_{Pt}}{d_{Pt}} \tanh\left(\frac{d_{Pt}}{2\lambda_{Pt}}\right) P_d, \qquad \text{(S.9)}$$

where $\rho$ is the resistivity of the Pt, $w = 5$mm is the distance between the probe electrodes attached to the Pt layer, $d_{Pt} = 10$nm is the thickness of the Pt layer, $\Theta_{SH} = 0.05$ is the spin Hall angle in Pt, $\lambda_{Pt} = 7.7$nm is the spin diffusion length in Pt, $e$ is the electron charge and $\hbar$ is the Planck constant.

It is important to note, that the value of the interface exchange integral $J_s$ and, correspondingly, the value of the surface energy density $E_s$ strongly depends on the method of fabrication of the sample and, therefore, can be measured only in an experiment performed for a particular sample.

To give a reasonable numerical example, below we take the value of $E_s$ as $E_s = 3.3 \cdot 10^{-3}\text{J/m}^2$, which was measured for the NiFe/NiO interface in [24].

For the given parameters, taking $\sin\theta = 0.01$, we obtain $V_{\text{ISHE}} = 40$mV for the *uncompensated* AFM boundary and $V_{\text{ISHE}} = 4$nV for the *compensated* one.

The reason for such a small magnitude of the ISHE voltage in the case of a *compensated* AFM interface is obvious. Since the dynamic magnetization $\mathbf{m}$ in the "compensated" case is $\gamma H_{ex}/\omega$ times smaller than the magnitude of the AFM vector $\mathbf{l}$, the energy of the exchange coupling $W_s$ at the FM/AFM interface in Eq.(2) is rather small.
